# Supplementary material for: Composite Active Learning: Towards Multi-Domain Active Learning with Theoretical Guarantees
Source: arXiv:2402.02110 source file (2024-02-03)
Supplement: Supplementary file 1 [file experiments.tex]

%mnist
\begin{table}[b]
% \vskip -0.7cm
\setlength{\tabcolsep}{0.5pt}
\caption{RotatingMNIST-D$6$ results ($\%$) for Vanilla (Vani.), CADOL-$\alpha$ (C.-$\alpha$), CADOL-FA (C.-FA), and CADOL. We mark the best result with \textbf{bold face} and the second-best results with \underline{underline}.}
\label{tab:rotatingmnist}
\tiny
\begin{center}
\begin{tabular}{l|cccc|cccc|cccc|cccc|cccc}
\toprule[1.5pt]
Query & \multicolumn{4}{c|}{Random \cite{al_survey}} & \multicolumn{4}{c|}{Margin \cite{margin}} & \multicolumn{4}{c|}{BADGE \cite{badge}} & \multicolumn{4}{c|}{Cluster-Margin \cite{cluster-margin}} & \multicolumn{4}{c}{Energy \cite{al4da_energy}} \\ \midrule
Method         & Vani.  & C.-$\alpha$  & C.-FA  & CAD. & Vani.  & C.-$\alpha$  & C.-FA  & CAD. & Vani.  & C.-$\alpha$  & C.-FA & CAD. & Vani.    & C.-$\alpha$    & C.-FA   & CAD.  & Vani.    & C.-$\alpha$    & C.-FA   & CAD.  \\ \midrule
Round 0       &49.2$_{\pm1.3}$&\underline{49.6}$_{\pm1.2}$&49.2$_{\pm1.5}$&\textbf{52.1}$_{\pm1.4}$&49.2$_{\pm1.3}$&\underline{49.6}$_{\pm1.2}$&49.2$_{\pm1.5}$&\textbf{52.1}$_{\pm1.4}$&49.2$_{\pm1.3}$&\underline{49.6}$_{\pm1.2}$&49.2$_{\pm1.5}$&\textbf{52.1}$_{\pm1.8}$&49.2$_{\pm1.3}$&\underline{49.6}$_{\pm1.2}$&49.2$_{\pm1.5}$&\textbf{52.1}$_{\pm1.4}$&49.2$_{\pm1.3}$&49.6$_{\pm1.2}$&\underline{49.9}$_{\pm1.1}$&\textbf{52.1}$_{\pm1.4}$\\ 
Round 1       &58.4$_{\pm0.5}$&58.7$_{\pm0.2}$&\underline{64.2}$_{\pm2.7}$&\textbf{70.2}$_{\pm1.0}$&59.3$_{\pm1.0}$&\underline{60.8}$_{\pm0.8}$&60.3$_{\pm2.0}$&\textbf{62.0}$_{\pm1.2}$&61.0$_{\pm0.2}$&59.3$_{\pm0.3}$&\underline{62.6}$_{\pm3.1}$&\textbf{71.2}$_{\pm1.6}$&58.7$_{\pm0.7}$&59.9$_{\pm1.6}$&\underline{60.9}$_{\pm0.7}$&\textbf{65.2}$_{\pm2.0}$&59.8$_{\pm0.7}$&\underline{60.5}$_{\pm0.6}$&58.9$_{\pm0.5}$&\textbf{62.2}$_{\pm0.7}$\\ 
Round 2       &64.5$_{\pm0.6}$&66.3$_{\pm0.5}$&\underline{74.2}$_{\pm0.7}$&\textbf{80.3}$_{\pm1.2}$&65.8$_{\pm0.8}$&67.1$_{\pm0.5}$&\underline{73.9}$_{\pm0.6}$&\textbf{76.0}$_{\pm1.0}$&66.2$_{\pm0.6}$&67.1$_{\pm1.1}$&\underline{74.1}$_{\pm1.1}$&\textbf{79.5}$_{\pm1.6}$&65.6$_{\pm1.5}$&68.0$_{\pm0.8}$&\underline{71.8}$_{\pm2.4}$&\textbf{74.9}$_{\pm1.6}$&64.7$_{\pm0.6}$&68.4$_{\pm2.2}$&\underline{73.0}$_{\pm1.6}$&\textbf{76.1}$_{\pm1.8}$\\ 
Round 3       &68.8$_{\pm0.8}$&73.3$_{\pm0.1}$&\underline{79.9}$_{\pm1.7}$&\textbf{85.0}$_{\pm0.8}$&70.6$_{\pm1.6}$&75.6$_{\pm1.4}$&\underline{80.0}$_{\pm1.4}$&\textbf{82.7}$_{\pm0.4}$&71.4$_{\pm1.1}$&73.9$_{\pm2.6}$&\underline{80.0}$_{\pm1.1}$&\textbf{85.4}$_{\pm0.5}$&70.0$_{\pm0.8}$&\underline{77.0}$_{\pm0.2}$&74.7$_{\pm1.0}$&\textbf{79.2}$_{\pm1.0}$&69.2$_{\pm1.9}$&74.6$_{\pm1.2}$&\underline{79.2}$_{\pm2.1}$&\textbf{81.9}$_{\pm1.8}$\\ 
Round 4       &77.7$_{\pm1.2}$&77.6$_{\pm0.9}$&\underline{83.4}$_{\pm0.7}$&\textbf{87.6}$_{\pm0.6}$&80.3$_{\pm0.2}$&80.8$_{\pm0.1}$&\underline{83.5}$_{\pm0.7}$&\textbf{84.3}$_{\pm1.7}$&80.5$_{\pm1.0}$&79.6$_{\pm0.8}$&\underline{81.5}$_{\pm0.9}$&\textbf{87.1}$_{\pm0.7}$&80.6$_{\pm0.5}$&\underline{81.1}$_{\pm0.4}$&79.6$_{\pm0.3}$&\textbf{81.6}$_{\pm0.6}$&80.1$_{\pm0.8}$&78.6$_{\pm0.7}$&\underline{82.1}$_{\pm1.0}$&\textbf{84.7}$_{\pm1.7}$\\ 
Round 5       &80.5$_{\pm0.7}$&80.8$_{\pm0.5}$&\underline{86.0}$_{\pm0.5}$&\textbf{88.7}$_{\pm0.3}$&83.1$_{\pm0.8}$&82.8$_{\pm0.6}$&\underline{85.4}$_{\pm0.7}$&\textbf{86.8}$_{\pm1.3}$&83.1$_{\pm0.2}$&82.4$_{\pm0.8}$&\underline{84.1}$_{\pm0.5}$&\textbf{88.3}$_{\pm0.6}$&\textbf{83.3}$_{\pm0.2}$&82.8$_{\pm0.8}$&81.3$_{\pm0.1}$&\underline{83.1}$_{\pm0.6}$&82.9$_{\pm0.1}$&81.4$_{\pm0.7}$&\underline{83.8}$_{\pm1.2}$&\textbf{85.8}$_{\pm1.0}$\\  \midrule
Average &66.5$_{\pm0.4}$&67.7$_{\pm0.5}$&\underline{72.8}$_{\pm0.4}$&\textbf{77.3}$_{\pm0.1}$&68.1$_{\pm0.3}$&69.5$_{\pm0.1}$&\underline{72.1}$_{\pm0.1}$&\textbf{74.0}$_{\pm0.8}$&68.6$_{\pm0.2}$&68.7$_{\pm0.9}$&\underline{71.9}$_{\pm1.1}$&\textbf{77.3}$_{\pm0.5}$&67.9$_{\pm0.5}$&\underline{69.7}$_{\pm0.3}$&69.6$_{\pm0.6}$&\textbf{72.7}$_{\pm0.7}$&67.6$_{\pm0.5}$&68.9$_{\pm0.7}$&\underline{71.1}$_{\pm0.9}$&\textbf{73.8}$_{\pm1.1}$\\ 
\bottomrule[1.5pt]
\end{tabular}
\end{center}
% \vskip -0.7cm
\end{table}

% Office-Home
\begin{table}[t]
\setlength{\tabcolsep}{0.5pt}
\caption{Office-Home results ($\%$) for Vanilla (Vani.), CADOL-$\alpha$ (C.-$\alpha$), CADOL-FA (C.-FA), and CADOL. We mark the best result with \textbf{bold face} and the second-best results with \underline{underline}.}
\label{tab:office-home}
\tiny
\begin{center}
\begin{tabular}{l|cccc|cccc|cccc|cccc|cccc}
\toprule[1.5pt]
Query & \multicolumn{4}{c|}{Random \cite{al_survey}} & \multicolumn{4}{c|}{Margin \cite{margin}} & \multicolumn{4}{c|}{BADGE \cite{badge}} & \multicolumn{4}{c|}{Cluster-Margin \cite{cluster-margin}} & \multicolumn{4}{c}{Energy \cite{al4da_energy}} \\ \midrule
Method         & Vani.  & C.-$\alpha$  & C.-FA  & CAD. & Vani.  & C.-$\alpha$  & C.-FA  & CAD. & Vani.  & C.-$\alpha$  & C.-FA & CAD. & Vani.    & C.-$\alpha$    & C.-FA   & CAD.  & Vani.    & C.-$\alpha$    & C.-FA   & CAD.  \\ \midrule
Round 0       &32.8 $\pm$1.0&\underline{33.5} $\pm$1.2&31.6 $\pm$2.3&\textbf{34.5} $\pm$1.3&32.8 $\pm$1.0&\underline{33.5} $\pm$1.2&31.6 $\pm$2.3&\textbf{34.5} $\pm$1.3&32.8 $\pm$1.0&\underline{33.5} $\pm$1.2&31.6 $\pm$2.3&\textbf{34.5} $\pm$1.3&32.8 $\pm$1.0&\underline{33.5} $\pm$1.2&31.6 $\pm$2.3&\textbf{34.5} $\pm$1.3&32.8 $\pm$1.0&\underline{33.5} $\pm$1.2&33.3 $\pm$1.3&\textbf{35.0} $\pm$1.9\\ 
Round 1       &42.8 $\pm$0.8&\underline{44.3} $\pm$1.6&43.5 $\pm$1.7&\textbf{45.2} $\pm$1.0&41.6 $\pm$1.2&42.4 $\pm$0.7&\underline{43.5} $\pm$0.5&\textbf{45.0} $\pm$0.8&42.6 $\pm$0.2&\underline{45.7} $\pm$0.7&44.6 $\pm$0.4&\textbf{47.0} $\pm$0.6&42.8 $\pm$0.6&\underline{43.0} $\pm$0.4&42.5 $\pm$0.5&\textbf{45.2} $\pm$1.5&41.2 $\pm$1.4&43.1 $\pm$1.3&\textbf{43.5} $\pm$2.0&\underline{43.3} $\pm$1.2\\ 
Round 2       &48.6 $\pm$0.5&\underline{50.9} $\pm$0.6&50.0 $\pm$1.8&\textbf{52.7} $\pm$1.8&46.6 $\pm$1.6&\underline{49.1} $\pm$1.0&48.6 $\pm$0.4&\textbf{50.4} $\pm$0.7&48.1 $\pm$0.8&50.5 $\pm$0.6&\underline{51.3} $\pm$0.9&\textbf{52.2} $\pm$1.3&47.0 $\pm$0.3&48.9 $\pm$0.7&\underline{49.4} $\pm$1.2&\textbf{51.9} $\pm$0.9&48.0 $\pm$0.9&49.5 $\pm$1.6&\underline{49.7} $\pm$0.8&\textbf{52.1} $\pm$0.6\\ 
Round 3       &52.6 $\pm$0.4&\underline{54.3} $\pm$0.7&54.2 $\pm$1.2&\textbf{56.1} $\pm$0.8&51.3 $\pm$0.6&\underline{54.1} $\pm$0.4&53.5 $\pm$0.8&\textbf{55.0} $\pm$1.0&52.0 $\pm$0.6&54.3 $\pm$0.8&\underline{54.6} $\pm$1.0&\textbf{57.2} $\pm$0.6&50.6 $\pm$0.8&\underline{53.4} $\pm$1.6&51.6 $\pm$0.1&\textbf{54.2} $\pm$0.8&51.2 $\pm$0.6&53.0 $\pm$1.4&\underline{55.0} $\pm$0.5&\textbf{56.0} $\pm$0.9\\ 
Round 4       &\underline{57.6} $\pm$0.3&57.3 $\pm$0.5&57.2 $\pm$0.5&\textbf{59.2} $\pm$1.3&55.9 $\pm$0.4&57.0 $\pm$0.9&\underline{57.0} $\pm$1.3&\textbf{57.6} $\pm$1.3&57.1 $\pm$0.2&\underline{58.7} $\pm$0.8&57.0 $\pm$1.4&\textbf{59.6} $\pm$0.4&55.9 $\pm$1.1&\textbf{57.6} $\pm$0.3&56.0 $\pm$0.7&\underline{57.5} $\pm$2.1&56.0 $\pm$1.2&56.7 $\pm$0.5&\underline{58.3} $\pm$0.9&\textbf{58.9} $\pm$1.6\\ 
Round 5       &58.0 $\pm$0.7&\underline{59.2} $\pm$0.2&58.8 $\pm$0.8&\textbf{60.5} $\pm$0.1&57.7 $\pm$2.1&\underline{58.6} $\pm$1.1&57.2 $\pm$0.5&\textbf{59.2} $\pm$0.7&56.9 $\pm$0.8&\underline{59.4} $\pm$0.5&58.8 $\pm$0.4&\textbf{60.3} $\pm$0.1&57.5 $\pm$1.8&\textbf{59.1} $\pm$0.3&56.6 $\pm$0.7&\underline{58.9} $\pm$0.4&58.4 $\pm$1.4&58.7 $\pm$1.1&\underline{59.4} $\pm$0.6&\textbf{60.5} $\pm$0.6\\  \midrule
Average &48.7 $\pm$0.3&\underline{49.9} $\pm$0.6&49.2 $\pm$0.4&\textbf{51.4} $\pm$1.0&47.6 $\pm$0.9&\underline{49.1} $\pm$0.5&48.6 $\pm$0.2&\textbf{50.3} $\pm$0.6&48.2 $\pm$0.3&\underline{50.3} $\pm$0.6&49.6 $\pm$1.0&\textbf{51.8} $\pm$0.2&47.8 $\pm$0.8&\underline{49.3} $\pm$0.5&47.9 $\pm$0.6&\textbf{50.4} $\pm$1.0&47.9 $\pm$0.7&49.1 $\pm$0.9&\underline{49.9} $\pm$0.4&\textbf{51.0} $\pm$0.8\\ 
\bottomrule[1.5pt]
\end{tabular}
\end{center}
\vskip -0.7cm
\end{table}

% ImageCLEF
\begin{table*}
\setlength{\tabcolsep}{0.5pt}
\caption{ImageCLEF results ($\%$) for Vanilla (Vani.), CADOL-$\alpha$ (C.-$\alpha$), CADOL-FA (C.-FA), and CADOL. We mark the best result with \textbf{bold face} and the second-best results with \underline{underline}.}
\label{tab:ImageCLEF}
\tiny
\begin{center}
\begin{tabular}{l|cccc|cccc|cccc|cccc|cccc}
\toprule[1.5pt]
Query & \multicolumn{4}{c|}{Random \cite{al_survey}} & \multicolumn{4}{c|}{Margin \cite{margin}} & \multicolumn{4}{c|}{BADGE \cite{badge}} & \multicolumn{4}{c|}{Cluster-Margin \cite{cluster-margin}} & \multicolumn{4}{c}{Energy \cite{al4da_energy}} \\ \midrule
Method         & Vani.  & C.-$\alpha$  & C.-FA  & CAD. & Vani.  & C.-$\alpha$  & C.-FA  & CAD. & Vani.  & C.-$\alpha$  & C.-FA & CAD. & Vani.    & C.-$\alpha$    & C.-FA   & CAD.  & Vani.    & C.-$\alpha$    & C.-FA   & CAD.  \\ \midrule
Round 0       &39.4 $\pm$2.7&36.8 $\pm$2.7&\underline{41.2} $\pm$4.0&\textbf{41.7} $\pm$1.7&39.4 $\pm$2.7&37.1 $\pm$2.6&\underline{41.2} $\pm$4.0&\textbf{41.7} $\pm$1.7&39.4 $\pm$2.7&36.8 $\pm$2.7&\underline{41.2} $\pm$4.0&\textbf{41.7} $\pm$1.7&39.4 $\pm$2.7&37.1 $\pm$2.6&\underline{41.2} $\pm$4.0&\textbf{41.7} $\pm$1.7&39.4 $\pm$2.7&37.2 $\pm$2.6&\underline{41.2} $\pm$4.0&\textbf{41.7} $\pm$1.7\\ 
Round 1       &49.8 $\pm$2.1&49.9 $\pm$2.5&\underline{51.5} $\pm$2.7&\textbf{52.5} $\pm$1.5&\underline{58.8} $\pm$2.4&58.7 $\pm$2.5&57.2 $\pm$3.1&\textbf{60.0} $\pm$7.1&54.0 $\pm$3.4&\underline{56.3} $\pm$3.9&54.4 $\pm$0.8&\textbf{58.3} $\pm$3.1&52.2 $\pm$3.2&\textbf{57.9} $\pm$3.1&53.4 $\pm$2.0&\underline{56.5} $\pm$6.2&58.0 $\pm$3.9&\underline{60.3} $\pm$2.5&57.0 $\pm$4.8&\textbf{60.8} $\pm$1.9\\ 
Round 2       &57.8 $\pm$0.4&58.5 $\pm$0.2&\underline{60.3} $\pm$1.3&\textbf{62.6} $\pm$1.1&61.7 $\pm$4.6&\underline{63.5} $\pm$2.3&63.4 $\pm$1.6&\textbf{68.3} $\pm$3.2&58.5 $\pm$4.8&59.0 $\pm$3.7&\underline{61.6} $\pm$1.3&\textbf{67.8} $\pm$2.4&59.9 $\pm$0.9&61.0 $\pm$5.4&\underline{66.3} $\pm$1.2&\textbf{67.8} $\pm$2.4&63.3 $\pm$1.6&64.3 $\pm$2.1&\underline{66.0} $\pm$0.7&\textbf{69.2} $\pm$0.5\\ 
Round 3       &65.0 $\pm$2.5&65.9 $\pm$3.0&\underline{68.7} $\pm$2.6&\textbf{71.3} $\pm$3.7&69.0 $\pm$2.3&70.6 $\pm$1.9&\underline{73.2} $\pm$1.2&\textbf{73.8} $\pm$2.7&64.7 $\pm$4.3&65.9 $\pm$3.1&\textbf{72.2} $\pm$0.9&\underline{71.2} $\pm$1.9&65.6 $\pm$1.1&68.0 $\pm$5.1&\underline{70.4} $\pm$2.3&\textbf{71.9} $\pm$2.5&70.2 $\pm$1.1&69.0 $\pm$0.9&\underline{71.9} $\pm$1.0&\textbf{74.7} $\pm$1.7\\ 
Round 4       &69.8 $\pm$2.3&69.8 $\pm$2.5&\textbf{71.3} $\pm$2.0&\underline{71.0} $\pm$2.8&71.2 $\pm$1.4&71.9 $\pm$2.2&\textbf{73.3} $\pm$0.8&\underline{72.4} $\pm$2.7&68.0 $\pm$2.0&69.6 $\pm$1.9&\textbf{72.2} $\pm$2.3&\underline{71.2} $\pm$2.1&70.0 $\pm$1.8&\underline{72.6} $\pm$1.3&\textbf{73.3} $\pm$0.9&72.5 $\pm$1.9&\underline{72.7} $\pm$0.7&71.9 $\pm$0.5&71.5 $\pm$1.9&\textbf{73.5} $\pm$1.6\\ 
Round 5       &69.5 $\pm$2.3&71.5 $\pm$0.9&\underline{74.2} $\pm$2.7&\textbf{77.3} $\pm$2.7&71.5 $\pm$2.7&71.0 $\pm$3.9&\underline{75.8} $\pm$0.5&\textbf{77.8} $\pm$1.4&70.3 $\pm$2.7&71.0 $\pm$1.0&\textbf{75.8} $\pm$1.4&\underline{74.9} $\pm$2.2&71.0 $\pm$1.2&72.5 $\pm$1.2&\underline{73.8} $\pm$1.5&\textbf{78.8} $\pm$0.5&71.1 $\pm$1.6&73.0 $\pm$1.1&\underline{74.0} $\pm$1.2&\textbf{77.2} $\pm$1.7\\  \midrule
Average &58.6 $\pm$0.8&58.8 $\pm$0.4&\underline{61.2} $\pm$0.7&\textbf{62.7} $\pm$0.9&62.0 $\pm$2.4&62.1 $\pm$2.4&\underline{64.0} $\pm$1.2&\textbf{65.7} $\pm$2.3&59.2 $\pm$3.2&59.8 $\pm$1.6&\underline{62.9} $\pm$0.9&\textbf{64.2} $\pm$1.2&59.7 $\pm$1.4&61.5 $\pm$1.6&\underline{63.1} $\pm$1.0&\textbf{64.8} $\pm$1.5&62.5 $\pm$1.0&62.6 $\pm$1.2&\underline{63.6} $\pm$0.8&\textbf{66.2} $\pm$1.4\\ 
\bottomrule[1.5pt]
\end{tabular}
\end{center}
\vskip -0.7cm
\end{table*}

% Office-Caltech
\begin{table*}
\vskip -0.7cm
\setlength{\tabcolsep}{0.5pt}
\caption{Office-Caltech results ($\%$) for Vanilla (Vani.), CADOL-$\alpha$ (C.-$\alpha$), CADOL-FA (C.-FA), and CADOL. We mark the best result with \textbf{bold face} and the second-best results with \underline{underline}.}
\label{tab:Office-Caltech}
\tiny
\begin{center}
\begin{tabular}{l|cccc|cccc|cccc|cccc|cccc}
\toprule[1.5pt]
Query & \multicolumn{4}{c|}{Random \cite{al_survey}} & \multicolumn{4}{c|}{Margin \cite{margin}} & \multicolumn{4}{c|}{BADGE \cite{badge}} & \multicolumn{4}{c|}{Cluster-Margin \cite{cluster-margin}} & \multicolumn{4}{c}{Energy \cite{al4da_energy}} \\ \midrule
Method         & Vani.  & C.-$\alpha$  & C.-FA  & CAD. & Vani.  & C.-$\alpha$  & C.-FA  & CAD. & Vani.  & C.-$\alpha$  & C.-FA & CAD. & Vani.    & C.-$\alpha$    & C.-FA   & CAD.  & Vani.    & C.-$\alpha$    & C.-FA   & CAD.  \\ \midrule
Round 0       &50.0 $\pm$4.0&50.2 $\pm$4.2&\textbf{54.8} $\pm$4.5&\underline{53.0} $\pm$0.9&50.0 $\pm$4.0&50.2 $\pm$4.2&\textbf{54.8} $\pm$4.5&\underline{53.0} $\pm$0.9&50.0 $\pm$4.0&50.2 $\pm$4.2&\textbf{54.8} $\pm$4.5&\underline{53.0} $\pm$0.9&50.0 $\pm$4.0&50.2 $\pm$4.2&\textbf{54.8} $\pm$4.5&\underline{54.2} $\pm$3.7&50.0 $\pm$4.0&50.2 $\pm$4.2&\textbf{54.8} $\pm$4.5&\underline{51.7} $\pm$4.2\\ 
Round 1       &77.6 $\pm$1.9&\underline{78.6} $\pm$2.3&78.3 $\pm$2.0&\textbf{81.4} $\pm$1.1&72.5 $\pm$2.1&75.0 $\pm$2.6&\underline{77.3} $\pm$3.3&\textbf{78.1} $\pm$3.5&68.8 $\pm$3.4&72.3 $\pm$4.5&\underline{75.4} $\pm$3.1&\textbf{78.7} $\pm$2.7&69.0 $\pm$0.4&70.2 $\pm$8.2&\underline{75.0} $\pm$5.1&\textbf{77.5} $\pm$6.0&74.5 $\pm$4.0&71.6 $\pm$2.2&\underline{78.8} $\pm$6.4&\textbf{81.1} $\pm$1.3\\ 
Round 2       &80.9 $\pm$2.1&\underline{83.3} $\pm$2.0&82.5 $\pm$4.2&\textbf{86.1} $\pm$2.4&81.7 $\pm$2.1&\underline{84.8} $\pm$1.3&84.2 $\pm$4.2&\textbf{88.3} $\pm$1.7&78.9 $\pm$0.6&80.4 $\pm$1.2&\underline{83.7} $\pm$2.2&\textbf{87.9} $\pm$0.8&81.1 $\pm$1.2&82.6 $\pm$3.0&\underline{83.2} $\pm$5.0&\textbf{87.4} $\pm$3.3&82.9 $\pm$2.7&\underline{85.0} $\pm$2.0&81.9 $\pm$2.8&\textbf{86.3} $\pm$3.3\\ 
Round 3       &85.3 $\pm$1.0&87.0 $\pm$0.4&\textbf{88.4} $\pm$2.1&\underline{88.2} $\pm$2.3&86.3 $\pm$3.9&89.8 $\pm$1.4&\underline{90.7} $\pm$2.1&\textbf{91.4} $\pm$1.4&87.7 $\pm$1.2&89.1 $\pm$0.5&\underline{91.9} $\pm$0.5&\textbf{92.5} $\pm$1.2&\underline{87.8} $\pm$2.1&85.1 $\pm$3.7&87.8 $\pm$3.2&\textbf{93.2} $\pm$1.0&87.9 $\pm$1.5&89.7 $\pm$2.0&\underline{90.8} $\pm$0.7&\textbf{91.6} $\pm$2.2\\ 
Round 4       &88.4 $\pm$2.7&88.7 $\pm$0.8&\underline{88.7} $\pm$2.3&\textbf{89.1} $\pm$2.5&91.5 $\pm$1.2&\underline{92.6} $\pm$0.8&92.4 $\pm$1.0&\textbf{93.4} $\pm$0.4&91.7 $\pm$1.0&91.4 $\pm$1.2&\textbf{92.6} $\pm$0.5&\underline{92.5} $\pm$0.8&90.4 $\pm$2.3&89.4 $\pm$3.2&\underline{91.7} $\pm$0.6&\textbf{92.0} $\pm$0.0&90.3 $\pm$0.6&\underline{92.2} $\pm$0.5&91.5 $\pm$1.4&\textbf{92.3} $\pm$1.0\\ 
Round 5       &90.4 $\pm$0.9&89.7 $\pm$1.5&\underline{92.9} $\pm$0.0&\textbf{93.0} $\pm$1.7&91.0 $\pm$0.2&91.3 $\pm$0.4&\underline{93.3} $\pm$0.6&\textbf{93.6} $\pm$1.3&92.4 $\pm$0.6&91.2 $\pm$0.2&\underline{93.6} $\pm$0.3&\textbf{93.9} $\pm$0.4&89.3 $\pm$0.6&\underline{91.3} $\pm$0.9&90.8 $\pm$0.9&\textbf{94.3} $\pm$0.9&91.0 $\pm$0.6&92.3 $\pm$0.9&\underline{93.7} $\pm$1.2&\textbf{94.1} $\pm$0.4\\  \midrule
Average &78.8 $\pm$0.7&79.6 $\pm$0.4&\underline{81.0} $\pm$1.2&\textbf{81.8} $\pm$1.4&78.8 $\pm$1.7&80.6 $\pm$0.5&\underline{82.1} $\pm$2.5&\textbf{83.0} $\pm$0.7&78.3 $\pm$0.6&79.1 $\pm$1.3&\underline{82.0} $\pm$0.5&\textbf{83.1} $\pm$0.7&77.9 $\pm$1.4&78.1 $\pm$3.7&\underline{80.5} $\pm$2.5&\textbf{83.1} $\pm$2.2&79.4 $\pm$1.1&80.2 $\pm$1.5&\underline{81.9} $\pm$1.7&\textbf{82.9} $\pm$1.8\\ 
\bottomrule[1.5pt]
\end{tabular}
\end{center}
\end{table*}
%--------------

%-------------

% % Ablation on RotatingMNIST
% \begin{wraptable}{r}{5.4cm}
% \vskip -1.6cm
% % \begin{table}[t]
% \setlength{\tabcolsep}{2pt}
% \caption{Ablation study. OA represents Optimal Assignment. $3^{rd}$ and $2^{nd}$ are the third term and the second domain-gap term of~\eqnref{eq:objective}} respectively.
% \label{table:ablation}
% \scriptsize
% \begin{center}
% \begin{tabular}{l|ccccc}
% \toprule[1.5pt]
% Method         &CAD.&w/o OA &w/o $3^{rd}$ &w/o $2^{nd}$ &Vani.\\ \midrule
% Round 0       &\textbf{52.1}&52.1&49.7&49.6&49.2\\
% Round 1       &\textbf{70.2}&67.6&68.6&58.8&58.4\\
% Round 2       &\textbf{80.3}&80.0&79.2&66.4&64.5\\
% Round 3       &\textbf{85.0}&84.9&82.2&73.4&68.8\\
% Round 4       &\textbf{87.6}&87.4&85.8&77.1&77.7\\
% Round 5       &\textbf{88.7}&88.5&87.6&79.6&80.5\\ \midrule
% Average &\textbf{77.3}&76.8&75.5&67.5&66.5\\ \midrule
% \bottomrule[1.5pt]
% \end{tabular}
% \end{center}
% % \end{table}
% \vskip -0.6cm
% \end{wraptable}

% The change of average accuracy with the increasing number of domains on RotationMNIST
% \begin{table}[t]
% \setlength{\tabcolsep}{2pt}
% \caption{The change of average accuracy with the increasing number of domains}
% \label{table:rotationmnist}
% \footnotesize
% \begin{center}
% \begin{tabular}{c|ccc}
% \toprule[1.5pt]
% Number&CADOL-FA - Pure&CADOL - CADOL-FA&CADOL - CADOL-alpha\\ \midrule
% 2       &5.6&4.2&8.2\\
% 6       &6.3&4.5&9.6\\
% 30       &4.8&5.3&8.3\\
% 50       &5.0&5.9&10.0\\
% 150       &5.2&7.7&10.3\\
% \bottomrule[1.5pt]
% \end{tabular}
% \end{center}
% \end{table}
