# Supplementary material for: Composite Active Learning: Towards Multi-Domain Active Learning with Theoretical Guarantees
Source: arXiv:2402.02110 source file (2024-02-03)
Supplement: Supplementary file 2 [file intro_backup.tex]

\section{Introduction}
One of bottlenecks that prevents unleashing the full potential of machine learning in practical applications is data labeling. 
In the real world, unlabeled data can often be obtained easily. But data labeling is tedious, expensive and in some cases even not possible, if the volume of data is enormous or data are generated continually.
%, e.g., billions of images without labels are uploaded to the internet. Limited budget does not allow to label all unlabeled data which users could get. To mitigate this problem, the aim of active learning (AL) is to maximize the knowledge that one could extract from available labeled data.
To mitigate this problem, the aim of active learning (AL) is to maximize the knowledge that one could extract from limited labeled data so as to improve performance as high as possible. Specifically, existing AL methods mainly leverage query strategies to select and label unlabeled samples that are believed to be most beneficial for improving model performance, e.g., samples with high uncertainty. With the same labeling budget, active learning can lead to better performance compared to randomly selecting unlabeled data. 

%  due to the distribution shift across domains
Mainstream AL research has focused on applications in single-domain data and thus put more effort on query strategies to select more useful data, but plenty of real-world tasks operate on data from multiple domains, e.g., financial transactions and medical records generated from different companies or hospitals \cite{federated_learning}. 
% Examples include domains with continuous indices, e.g., disease diagnosis of patients across different ages, and domains with discrete indices, e.g., photos of wild animals taken by different cameras [CIDA]. 
However, active learning in the case of multi-domain data faces brand-new challenges. 1) Labeled data from one domain can be useful for other domains especially those who are similar to this domain, which is not needed to consider in single-domain active learning \cite{cida}. For example, in disease diagnosis of patients of ages, labeling more data of middle ages should be beneficial to data of both the young and the old \cite{cida}. Such benefit can be gotten by taking advantages of known inherent relationships among all domains. However, such relationships are hard to be gotten, particularly for domains with discrete indices. Moreover, especially, relationships are more difficult to be qualified, even when related relationships are known, e.g., domains with continuous indices. Therefore, how to discover inherent relationships and quantify them should be exploited in active learning.  2) Active learning in a single domain implicitly assumes that data points come from the same distribution. But multiple domains experience distribution shift across domain. In addition, there exists a negligible domain gap between labeled data of each domain and the domain itself and thus labeled data can be treated as a different domain for its original domain, since labeled data are too few to represent the original domain and query strategies bring various biases to the distribution of the labeled domain \cite{da4al_1, da4al_2}.
This makes it harder to evaluate the benefit of a labeled datum and to train models with good cross-domain generalization. 
For example, current query strategies, simply adapted to financial transactions across different companies, are not likely to yield best performance without considering the distribution discrepancies across origin domains and labeled domains. 

% because they do not take advantage of the inherent relationships and the distribution discrepancies across domains. 
 


 




 
%Although domains with discrete indexes do not have so explicit relationship like domains with continuous indexes, both two kinds of domains do not have quantified values of relationships among all domains, which thus cannot be directly adapted to multi-domain data in the AL setting.



TODO: and mention the solutions and then mention we have a upper bound, which we optimize to simultaneously enforcing our two solutions

\jie{The following paragraph should be expanded to explain the novelty of this paper.}

To overcome two fresh obstacles in AL, we propose a novel idea to both capture inherent relationships and reduce domain shift across all domains. Firstly, in order to quantify domain relationships between labeled domains and original domains, we advise to seek a most similar domain made up of weighted labeled domains for each origin domain, where weights are optimal when the domain gap is optimized to the smallest between the mixture domain and the original domain. The weight (named as importance score) of a labeled domain means the importance of the labeled domain to the origin domain and thus relationships are quantified implicitly. In this way, label assignment could utilize the sum of the importance score of a labeled domain to each original domain, i.e., the bigger the total score is, the more labeling budget that labeled domain should be assigned to. Simultaneously, the most similar mixture domain could be also as the surrogate domain to replace the origin domain in training. Secondly, although surrogate domains are gotten by discovering domain relationships, there may be still large domain gaps between surrogate domains and original domains, due to big domain gaps between original domains and labeled domains that constitute surrogate domains. Therefore, we suggest to align features between surrogate domains and labeled domains to further close domain gaps. Lastly, the discovery of relationships and feature alignment could be benefit to each other mutually. Accurate 
quantification to describe inherent relationships helps improve the importance of labeled domains with the closer link to an original domain, which stimulates feature alignment. Correspondingly, feature alignment between original domains and surrogate domains aligns supports between original domains and labeled domains, and similar supports facilitate us to find surrogate domains with smaller domain gap to origin domains so as to learn relationships more accurately. Therefore, formally, we propose a upper bound of the total error of all original domains, which we optimize to simultaneously enforce the quantification of relationships and the optimization of discrepancies among domains. 


% we firstly note that there exists a negligible domain-gap between labeled data in a domain and all data in this domain and thus labeled data can be treated as a new domain, since labeled data are too few to represent original domain and different query strategies bring various biases to the distribution of labeled data [da for al]. To explicitly quantify relationships between original domains and labeled domains, we propose to find the most similar surrogate domain with labels to represent an original domain to participate in training. The surrogate domain is made up of weighted labeled domains and the weights of labeled domains are optimized by reducing domain gap between the surrogate domain and its original domain, because most of data of original domains lack of labels. The weight of each labeled domain could be treated as importance of the labeled domain to the original domain. In this way, the "existed" relationships between labeled domains and original domains are "discovered". In order to "enhance" "current" relationship between the original domain and surrogate domain, i.e., make the two domains more similar, we propose to align the two domains by optimizing their features. To summary up, we propose to "discover existed" relationships between labeled domains and original domains by optimizing importance of labeled domains to original domains and to "enhance current" relationships between surrogate domains and original domains by optimizing their features. 

Our contributions are as follows:
\begin{itemize}
    \item We identify the problem of Multi-Domain Active Learning and propose Voting for Important Domains (VIDO) as the first general AL method for addressing this problem. Further, we analyze our method and provide theoretical guarantees that VIDO performs better than the state-of-the-art (SOTA) AL baselines due to its lower upper bound for average error of all domains.

\item We derive two variants of VIDO, VIDO-alpha and VIDA-FA, and both of them are also achieve improvement compared with SOTA AL baselines in theories.

\item We provide empirical results using both synthetic and real-world medical datasets with detailed ablation study,  which shows that VIDO and its two variants significantly improve performance over the state-of-the-art AL methods for Multi-Domain Active Learning.
\end{itemize}



% \begin{align}
% & \min_{h, e_h, e_f, \{h_i\}_{i=1}^N, \alpha} \max_{f} E(h, e_h, e_f, \{h_i\}_{i=1}^N, \alpha, d)
% \\
% &
%  =  \min_{h, e_h, e_f, \{h_i\}_{i=1}^N, \alpha} \max_{f} \sum_{j=1}^N  \frac{\alpha_{j}}{N_j^l}\sum_{k=1}^{N_j^l} L_Y(h \circ e_h(x_{j,k}^l), y_{j, k}^l) 
% \\
% &
% - \frac{\lambda_d}{2N}\sum_{i=1}^N [\frac{1}{N_i}\sum_{k=1}^{N_i} L_D(f \circ e_f(x_{i,k}), y^{\mathcal{O}}=1)+\sum_{j=1}^N \frac{\alpha_{i,j}}{N_j^l} \sum_{k=1}^{N_j^l} L_D(f \circ e_f(x_{j,k}^l), y^{\mathcal{S}}=0)]
% \\
% &
% +   \frac{1}{N}\sum_{i=1}^N \sum_{j=1}^N \frac{\alpha_{i, j}}{N_j^l} \sum_{k=1}^{N_j^l} L_Y(h_i \circ e_h(x_{j,k}^l), y_{j, k}^l) 
% \\
% &
% =   \min_{h, e_h, e_f, \{h_i\}_{i=1}^N, \alpha} \max_{f} \sum_{j=1}^N  \frac{\alpha_{j}}{N_j^l}\sum_{k=1}^{N_j^l} L_Y^{j, k}(h, e_h)
% \\
% &
% + \frac{\lambda_d}{2N}\sum_{i=1}^N [\frac{1}{N_i}\sum_{k=1}^{N_i} L_D^{i, k}(e_f, \alpha, d)+\sum_{j=1}^N \frac{\alpha_{i,j}}{N_j^l} \sum_{k=1}^{N_j^l} L_D^{j,k}(e_f, \alpha, d)]
% \\
% &
% +   \frac{1}{N}\sum_{i=1}^N \sum_{j=1}^N \frac{\alpha_{i, j}}{N_j^l} \sum_{k=1}^{N_j^l} L_Y^{j, k}(h_i, e_h)
% \label{vid\mathcal{O}_loss}
% \end{align}

% \begin{align}
% & \min_{h, e_h, e_f, \{h_i\}_{i=1}^N, \alpha} \max_{f} E(h, e_h, e_f, \{h_i\}_{i=1}^N, \alpha, d)
% \\
% &
%  =   \min_{h, e_h, e_f, \{h_i\}_{i=1}^N, \alpha} \max_{f} \sum_{j=1}^N  \alpha_{j} \mmathbb{E}^{\mathcal{L}_j} [L_Y(h \circ e_h(x), y)] 
% \\
% &
% - \frac{\lambda_d}{2N}\sum_{i=1}^N \{ \mmathbb{E}^{\mathcal{O}_i} [L_D(f \circ e_f(x), y^{\mathcal{O}}=1)]+\sum_{j=1}^N \alpha_{i,j} \mmathbb{E}^{\mathcal{L}_j} [L_D(f \circ e_f(x), y^{\mathcal{S}}=0)] \}
% \\
% &
% +   \frac{1}{N}\sum_{i=1}^N \sum_{j=1}^N \alpha_{i, j} \mmathbb{E}^{\mathcal{L}_j} [L_Y(h_i \circ e_h(x), y)] 
% \label{vid\mathcal{O}_loss}
% \end{align}

% &\min_{h, e_h, e_f, \{h_i\}_{i=1}^N, \alpha} \max_{f} E(h, e_h, e_f, \{h_i\}_{i=1}^N, \alpha, d)
% \\
% &
% = 

\begin{equation}
\begin{aligned}
 \min_h & \quad \frac{1}{N} \sum_j (\sum_i \alpha_{i, j}^*) \epsilon_{\mathcal{L}_j}(h) + \frac{1}{N}\sum_i \frac{1}{2} d_{\mathcal{H}\Delta \mathcal{H}}({\mathcal{O}_i(Z)}^*, \sum_j \alpha_{i, j}^* {\mathcal{L}_j(Z)}^*) + \frac{1}{N} \sum_i \lambda_{i}
\\
s.t. & \quad \sum_i \alpha_{i, j}^*=1, j=1,2,.., N, \tag{a} 
\\
& \quad
{D(Z)}^*,  {D^l(Z)}^* = {D(Z)},  {D^l(Z)} \text{ when } h, e = arg \min_{h}  \frac{1}{N} \sum_j (\sum_i \alpha_{i, j}^*) \epsilon_{\mathcal{L}_j}(h)
\\
& \quad
{\alpha}^* = arg \min_\alpha  \frac{1}{N}\sum_i \frac{1}{2} d_{\mathcal{H}\Delta \mathcal{H}}({\mathcal{O}_i(Z)}^*, \sum_j \alpha_{i, j} {\mathcal{L}_j(Z)}^*) + \frac{1}{N} \sum_i \lambda_{i}
\end{aligned}
\end{equation}
where the three conditions ensure that the upper bound of baselines becomes tightest in the form of our upper-bound theory. \hao{To revise. Consider removing this.}

% Office-Home
\begin{table}[t]
\setlength{\tabcolsep}{2pt}
\caption{Results on Office-Home}
\label{tab:Office-Home}
\scriptsize
\begin{center}
\begin{tabular}{l|cccc|cccc|cccc|cccc}
\toprule[1.5pt]
Query & \multicolumn{4}{c|}{Random} & \multicolumn{4}{c|}{Margin} & \multicolumn{4}{c|}{BADGE} & \multicolumn{4}{c}{Cluster-Margin} \\ \midrule
Method         & Vanilla  & $\alpha$  & FA  & CADOL & Vanilla  & $\alpha$  & FA  & CADOL & Vanilla  & $\alpha$  & FA & CADOL & Vanilla    & $\alpha$    & FA   & CADOL   \\ \midrule
Round 0       &32.8&\underline{33.5}&31.6&\textbf{34.5}&32.8&\underline{33.5}&31.6&\textbf{34.5}&32.8&\underline{33.5}&31.6&\textbf{34.5}&32.8&\underline{33.5}&31.6&\textbf{34.5}\\
Round 1       &42.8&\underline{44.3}&43.5&\textbf{45.2}&41.6&42.4&\underline{43.5}&\textbf{45.0}&42.6&\underline{45.7}&44.6&\textbf{47.0}&42.8&\underline{43.0}&42.5&\textbf{45.2}\\
Round 2       &48.6&\underline{50.9}&50.0&\textbf{52.7}&46.6&\underline{49.1}&48.6&\textbf{50.4}&48.1&50.5&\underline{51.3}&\textbf{52.2}&47.0&48.9&\underline{49.4}&\textbf{51.9}\\
Round 3       &52.6&\underline{54.3}&54.2&\textbf{56.1}&51.3&\underline{54.1}&53.5&\textbf{55.0}&52.0&54.3&\underline{54.6}&\textbf{57.2}&50.6&\underline{53.4}&51.6&\textbf{54.2}\\
Round 4       &\underline{57.6}&57.3&57.2&\textbf{59.2}&55.9&57.0&\underline{57.0}&\textbf{57.6}&57.1&\underline{58.7}&57.0&\textbf{59.6}&55.9&\textbf{57.6}&56.0&\underline{57.5}\\
Round 5       &58.0&\underline{59.2}&58.8&\textbf{60.5}&57.7&\underline{58.6}&57.2&\textbf{59.2}&56.9&\underline{59.4}&58.8&\textbf{60.3}&57.5&\textbf{59.1}&56.6&\underline{58.9}\\ \midrule
Average &48.7&\underline{49.9}&49.2&\textbf{51.4}&47.6&\underline{49.1}&48.6&\textbf{50.3}&48.2&\underline{50.3}&49.6&\textbf{51.8}&47.8&\underline{49.3}&47.9&\textbf{50.4}\\ \midrule
\bottomrule[1.5pt]
\end{tabular}
\end{center}
\end{table}

% Office-Home with energy
\begin{table}[t]
\setlength{\tabcolsep}{2pt}
\caption{Results on Office-Home}
\label{tab:Office-Home}
\scriptsize
\begin{center}
\begin{tabular}{l|cccc|cccc|cccc|cccc}
\toprule[1.5pt]
Query & \multicolumn{4}{c|}{Random} & \multicolumn{4}{c|}{Margin} & \multicolumn{4}{c|}{BADGE} & \multicolumn{4}{c}{Energy} \\ \midrule
Method         & Vanilla  & $\alpha$  & FA  & CADOL & Vanilla  & $\alpha$  & FA  & CADOL & Vanilla  & $\alpha$  & FA & CADOL & Vanilla    & $\alpha$    & FA   & CADOL   \\ \midrule
Round 0       &32.8&\underline{33.5}&31.6&\textbf{34.5}&32.8&\underline{33.5}&31.6&\textbf{34.5}&32.8&\underline{33.5}&31.6&\textbf{34.5}&32.8&\underline{33.5}&33.3&\textbf{35.0}\\
Round 1       &42.8&\underline{44.3}&43.5&\textbf{45.2}&41.6&42.4&\underline{43.5}&\textbf{45.0}&42.6&\underline{45.7}&44.6&\textbf{47.0}&41.2&43.1&\textbf{43.5}&\underline{43.3}\\
Round 2       &48.6&\underline{50.9}&50.0&\textbf{52.7}&46.6&\underline{49.1}&48.6&\textbf{50.4}&48.1&50.5&\underline{51.3}&\textbf{52.2}&48.0&49.5&\underline{49.7}&\textbf{52.1}\\
Round 3       &52.6&\underline{54.3}&54.2&\textbf{56.1}&51.3&\underline{54.1}&53.5&\textbf{55.0}&52.0&54.3&\underline{54.6}&\textbf{57.2}&51.2&53.0&\underline{55.0}&\textbf{56.0}\\
Round 4       &\underline{57.6}&57.3&57.2&\textbf{59.2}&55.9&57.0&\underline{57.0}&\textbf{57.6}&57.1&\underline{58.7}&57.0&\textbf{59.6}&56.0&56.7&\underline{58.3}&\textbf{58.9}\\
Round 5       &58.0&\underline{59.2}&58.8&\textbf{60.5}&57.7&\underline{58.6}&57.2&\textbf{59.2}&56.9&\underline{59.4}&58.8&\textbf{60.3}&58.4&58.7&\underline{59.4}&\textbf{60.5}\\ \midrule
Average &48.7&\underline{49.9}&49.2&\textbf{51.4}&47.6&\underline{49.1}&48.6&\textbf{50.3}&48.2&\underline{50.3}&49.6&\textbf{51.8}&47.9&49.1&\underline{49.9}&\textbf{51.0}\\ \midrule
\bottomrule[1.5pt]
\end{tabular}
\end{center}
\end{table}


% Ablation on RotatingMNIST
\begin{table}[t]
\setlength{\tabcolsep}{2pt}
\caption{Ablation study ($\%$) for CADOL {using RotatingMNIST-D$6$ and the Random strategy}. {OA means optimal assignment.} $2^{nd}$ and $3^{rd}$ denote the second and the third terms of~\eqnref{eq:objective}, respectively.}
\label{table:ablation}
\footnotesize
\begin{center}
\begin{tabular}{l|ccccc}
\toprule[1.5pt]
Method         &CADOL&w/o OA &w/o $2^{nd}$ &w/o $3^{rd}$ & Vanilla \\ \midrule
Round 0       &52.1&52.1&49.7&49.6&49.2\\
Round 1       &70.2&67.6&68.6&58.8&58.4\\
Round 2       &80.3&80.0&79.2&66.4&64.5\\
Round 3       &85.0&84.9&82.2&73.4&68.8\\
Round 4       &87.6&87.4&85.8&77.1&77.7\\
Round 5       &88.7&88.5&87.6&79.6&80.5\\ \midrule
Average &77.3&76.8&75.5&67.5&66.5\\ 
\bottomrule[1.5pt]
\end{tabular}
\end{center}
\vskip -0.9cm
\end{table}
%----------
